# Supplementary material for: "A Posteriori" Limited High Order and Robust Residual Distribution Schemes for Transient Simulations of Fluid Flows in Gas Dynamics
Source: arXiv:1902.07773 source file (2023-01-02)
Supplement: Supplementary file 1 [file Appendix.tex]

\section{Some well-known Propositions and Theorems for the Residual Distribution Schemes}\label{appendix:DMPLDA}

Consider a generic scalar conservation law, such as the linear advection problem given by
\begin{equation}\label{eq:scalar_advection}
\partial_t U+ \nabla \cdot \F(U)=0, \,\, \text{on}\,\, \Omega_h\subset \mathbb{R}^2 \times \mathbb{R}^{+},
\end{equation}
with $\F(U)=\mathbf{a}U$ and $\mathbf{a}=(a_1,a_2)\in \mathbb{R}^2$ constant or with $\nabla \cdot \mathbf{a}=0$.
Let us focus on continuous piecewise linear approximations, for which the discrete unknowns are the values of the solution in the vertices of the triangulation, with the notation as in figure \ref{fig:notation} and take the semi-discrete form of the scheme
\begin{equation}\label{scalar_ode}
|C_i|\frac{dU_i}{dt}+\sum_{K \in \mathcal{K}_i} \phi_i^K, \, \forall i \in \Omega_h,
\end{equation}
with the nodal residual written as 
\begin{equation}
\phi_i=\sum_{j\in K, j\neq i} c_{ij}(U_i-U_j).
\end{equation}
The coefficients $c_{ij}$ are subject to conditions, which guarantee the existence of a discrete maximum principle. 

\subsection{The Local Extremum Diminishing Principle (LED)}\label{app:LED}
Following \cite{Ricchiuto2007}, the generic scheme \eqref{scalar_ode} has the property of Local Extremum Diminishing (LED) in case the coefficients $c_{ij}$ fulfil 
\begin{equation}\label{LED_property}
\sum_{K \in \mathcal{K}_i \cap \mathcal{K}_j} c_{ij} \geq 0, \, \forall j\in \mathcal{K}_i, \, j \neq i \, \text{and} \, \forall i\in \Omega_h,
\end{equation}
which guarantees that local minima and local maxima are bounded .

The requirement of $c_{ij} \geq 0$ $\forall j \in K$ and $\forall K \in \mathcal{K}_i$ is generally referred to as a ''Sub-element LED``.

\subsection{The Discrete Maximum Principle (DMP)-Monotonicity}\label{app:DMP}
The global discrete space-time maximum principle $$U_{min}^n=\min_{j\in \Omega_h} U_j^n \leq U_{i}^{n+1}\leq \max_{j\in \Omega_h}=U_{max}^n$$
and the local DMP given by $$\overline{U}_i=\min\{U_i^n, \min_{j \in \mathcal{K}_i,j \neq i} (U_j^n, U_j^{n+1})\} \leq U_i^{n+1}\leq  \max\{U_i^n, \max_{j \in \mathcal{K}_i,j \neq i} (U_j^n, U_j^{n+1})\} = \overline{U}_i$$
are verified, if the LED condition \eqref{LED_property} holds together with an opportune time-step restriction dictated by the chosen method.
This scheme fulfils the Local Extremum Diminishing principle at a sub-element level, if $c_{ij}^K\geq 0,\,\forall i,j$. 
Monotonicity for the iterative method \eqref{eq:defcor} will be then preserved, if a CFL-condition $$\Delta t \max_{K,i \in K}\left( \frac{\sum_{j \in K}c_{ij}^K}{|K|}\right) \leq 1.$$
Of course, it is important to remind, that monotonicity can be shown on a scalar problem, whereas, in case of systems, one should rely on rather on intuition.

\subsection{Lax-Wendroff theorem for Residual Distribution schemes}\label{app:LaxWendrTH}
The Lax-Wendroff theorem, proven in \cite{Abgrall2001}, states that, 
given some bounded initial data $U_0\in \mathcal{L}_\infty (\mathbb{R}^2)$, a square integrable function $u\in  \mathcal{L}_\infty (\mathbb{R}^2 \times \mathbb{R^{+}})$ and a constant $C$ which depends on the initial data $U_0$ and on $U$ such that the approximation $U_h(\mathbf{x},t)$ given by the definition of the residual distribution scheme \eqref{eq:residual}-\eqref{eq:phicons} fulfils
\begin{equation}\label{LxW_theorem}
\sup_h \sup_{(\mathbf{x}, t)} |U_h| \leq C \quad \text{and}\quad  \lim_{h\rightarrow 0}||U_h-U||_{\mathcal{L}_2^{loc}(\mathbb{R}^2\times \mathbb{R}^+)}=0,
\end{equation}
then U is a weak solution to the problem.
